# Supplementary material for: Regional-Local Adversarially Learned One-Class Classifier Anomalous Sound Detection in Global Long-Term Space
Source: arXiv:2202.13245 source file (2022-02-26)
Supplement: Supplementary file 2 [file FlowSatus.tex]

\begin{table}[htbp]
\centering
\caption{Cavitation datasets content details.}
\label{tab: CavitationDatasets-FlowStatus}
\small
\setlength{\tabcolsep}{0.3mm}{
\begin{tabular}{lccccc}
\toprule 
\multirow{2}{*}{Dataset} & \multicolumn{3}{c}{Abnormal} & \multicolumn{2}{c}{Normal}  \\ 
\cmidrule{2-6} 
& \multicolumn{1}{l}{choked flow} & \multicolumn{1}{l}{constant} & \multicolumn{1}{l}{incipient} & \multicolumn{1}{l}{turbulent} & \multicolumn{1}{l}{no flow} \\ 
\midrule
Cavitation2017           & 72    & 93   & 40   & 118   & 33  \\ 
Cavitation2018           & 148   & 396  & 64   & 183   & 15  \\ 
Cavitation2018-noise     & 40    & 40   & 40   & 40    & 0  \\ 
\bottomrule
\end{tabular}}
\end{table}
