# Supplementary material for: Regional-Local Adversarially Learned One-Class Classifier Anomalous Sound Detection in Global Long-Term Space
Source: arXiv:2202.13245 source file (2022-02-26)
Supplement: Supplementary file 3 [file MIMII_training_test.tex]

\begin{table}[htbp]
\centering
\caption{Details of the training and test sets on MIMII.}
\label{tab: MIMII training and test sets}
\footnotesize
\setlength{\tabcolsep}{0.8mm}{
\begin{tabular}{cccc}
\toprule 
\multicolumn{2}{l}{Machine type / model ID} & Training set & Test set \\ 
\midrule
\multirow{4}{*}{Valve}            & 00      & 872          & 238      \\
                                  & 02      & 588          & 240      \\
                                  & 04      & 880          & 240      \\
                                  & 06      & 872          & 240      \\ 
\midrule
\multirow{4}{*}{Pump}             & 00      & 863          & 286      \\
                                  & 02      & 894          & 222      \\
                                  & 04      & 602          & 200      \\
                                  & 06      & 934          & 204      \\ 
\midrule
\multirow{4}{*}{Fan}              & 00      & 604          & 814      \\
                                  & 02      & 657          & 718      \\
                                  & 04      & 685          & 696      \\
                                  & 06      & 654          & 722      \\ 
\midrule
\multirow{4}{*}{Slide rail}       & 00      & 712          & 712      \\
                                  & 02      & 801          & 534      \\
                                  & 04      & 356          & 256      \\
                                  & 06      & 445          & 178      \\ 
\bottomrule
\end{tabular}
}
\end{table}
