# Supplementary material for: Regional-Local Adversarially Learned One-Class Classifier Anomalous Sound Detection in Global Long-Term Space
Source: arXiv:2202.13245 source file (2022-02-26)
Supplement: Supplementary file 5 [file cavitation_training_test.tex]

% Please add the following required packages to your document preamble:
% \usepackage{multirow}
\begin{table}[htbp]
\centering
\caption{Details of the training and test sets. $(\cdot )$ denotes the number after the sliding window (window size is 466944).}
\label{tab: training and test sets}
\footnotesize
\setlength{\tabcolsep}{0.05mm}{
\begin{tabular}{llcccccc}
\toprule 
\multicolumn{1}{c}{\multirow{3}{*}{Dataset}} & \multirow{3}{*}{Train}  & \multicolumn{6}{c}{Test}  \\ 
\cmidrule{3-8} 
\multicolumn{1}{c}{}&& \multicolumn{1}{l}{\multirow{2}{*}{Non-cavitation}} & \multicolumn{5}{c}{Cavitation (\%)}\\ 
\cmidrule{4-8} 
\multicolumn{1}{c}{}&  & \multicolumn{1}{l}{} & \multicolumn{1}{l}{10\%} & \multicolumn{1}{l}{20\%} & \multicolumn{1}{l}{30\%} & \multicolumn{1}{l}{40\%} & \multicolumn{1}{l}{50\%} \\ 
\midrule
Cavitation2017 & \multicolumn{1}{c}{121 (1210)} & 30 (300)  & 3 (30)  & 6 (60) & 12 (120)  & 20 (200)  & 30 (300)           \\
Cavitation2018 & \multicolumn{1}{c}{158 (13114)} & 40 (3320)  & 4 (332)  & 10 (830) & 17 (1411)  & 26 (2158)  & 40 (3320)   \\
Cavitation2018-noise& \multicolumn{1}{c}{32 (2656)}  & 8 (664)  & 1 (83) & 2 (166)  & 3 (249)  & 5 (415)  & 8 (664)         \\ 
\bottomrule
\end{tabular}
}
\end{table}
