# Supplementary material for: Regional-Local Adversarially Learned One-Class Classifier Anomalous Sound Detection in Global Long-Term Space
Source: arXiv:2202.13245 source file (2022-02-26)
Supplement: Supplementary file 6 [file results_different_SNR.tex]

\begin{table}[htbp]
\centering
\caption{AUC and ${F}_{1}$ score results for different intensity noise.}
\label{tab: results different SNR}
\footnotesize
\footnotesize
\setlength{\tabcolsep}{1mm}{
\begin{tabular}{cccccccc}
\toprule 
\multirow{2}{*}{Results} & \multicolumn{7}{c}{Different intensity noise (dB)} \\ 
\cmidrule{2-8} 
                         & -6   & -4   & -2   & 0  & 2  & 4  & 6  \\ 
\midrule 
AUC                      & 0.9753  & 0.9747  & 0.9756  & 0.9750   & 0.9756   & 0.9657  & 0.9748    \\
F1 score                 & 0.9831  & 0.9699  & 0.9831  & 0.9633   & 0.9831   & 0.9616  & 0.9699   \\ 
\bottomrule
\end{tabular}
}
\end{table}
